# Supplementary material for: Sintel: A Machine Learning Framework to Extract Insights from Signals
Source: arXiv:2204.09108 source file (2022-04-19)
Supplement: Supplementary file 1 [file appendix.tex]

\section*{Appendix}

\section{Database}
\label{sec:db}
The database stores all necessary information for the system. This includes the found anomalies and any outputs from the anomaly detection pipelines. Furthermore, we store any annotations that the user of the system might give through the visual interface.

Figure \ref{fig:db} shows the database collections and how they are related.

The database is implemented in mongoDB and allows flexibility and scalability. 

We store a total of seven collections. 

\paragraph{Signal} Signal is the collection where the different time series signals are stored. Note that we do not store any raw data in the database, but rather a link to the data location. Also, we store a reference to the Dataset collection. Additionally, we store metadata about the signal such as name, start and end time and in which columns the timestamps and values are located.

\paragraph{Dataset} Within the Dataset collection we only have a name field for the dataset. However, as we store the reference to the Dataset collection within Signal, a Dataset can be understood as a set of signals. This way we can group signals to datasets and run pipelines on these sets.

\paragraph{PipelineTemplate} The PipelineTemplate collection contains all the pipeline templates from which the pipelines that later on will be used to run an experiments are generated. The template includes all the default hyperparameter values, as well as the tunable hyperparameter ranges.

\paragraph{Pipeline} The Pipeline collection stores the pipeline JSON file, as required by MLPrimitives. Each pipeline is related to one PipelineTemplate and defines the specific hyperparameters that should be used.

\paragraph{Experiment} As we already defined, an experiment is a the application of a pipeline on a Dataset. Therefore an experiment is linked to the Dataset collection and the PipelineTemplate collection. Furthermore we add a project name to the experiment such that we are able to group experiments based on project names. Optionally a signalset can be specified, which can be a subset of the associated Dataset.

\paragraph{Datarun} The Datarun objects represent single executions of an Experiment, and contain all the information about the environment and context where this execution took place, which potentially allows to later on reproduce the results in a new environment.
It also contains information about whether the execution was successful or not, when it started and ended, and the number of events that were found in this experiment.

\paragraph{Signalrun} The Signalrun objects represent single executions of a Pipeline on a Signal within a Datarun.
It contains information about whether the execution was successful or not, when it started and ended, the number of events that were found by the Pipeline, and where the model and metrics are stored.

\paragraph{Event} In the event collection all details regarding found anomalies are stored. The events have a reference to the Signalrun and contain a start-time, end-time and score field.

\paragraph{Event Interaction} The Event Interaction collection records all the interaction history related to events.

\paragraph{Annotation} Each Event can have multiple Annotations, from one or more users. Annotations are expected to be inserted by the domain experts after the Datarun has finished and they analyze the results.

\begin{figure}
    \centering
    \begin{subfigure}[T]{0.8\linewidth}
    \inputminted[]{python}{listings/orex_api.py}
    \end{subfigure}
    \caption{Using python SDK. \texttt{OrionDBExplorer} allows users to run experiments and store them in the database as well as query and retrieve information from the database.}
\label{fig:orex-api}
\end{figure}

\section{Reproducibility}
This section contains more information about some implementation details of \textit{Orion}.

\subsection{Primitives}

\begin{table}[ht]
    \centering
    \begin{tabular}{l|c}
         \toprule
         Type            & Count \\
         \midrule
         Pre-processing  & 8 \\
         Modeling        & 6 \\
         Post-processing & 4 \\
         \bottomrule
    \end{tabular}
    \caption{Primitives in the curated catalog of the source library categorized by its type.}
    \label{tab:primitives_by_type}
\end{table}

\subsection{Pipelines}

\begin{figure}[ht]
\includegraphics[width=\linewidth]{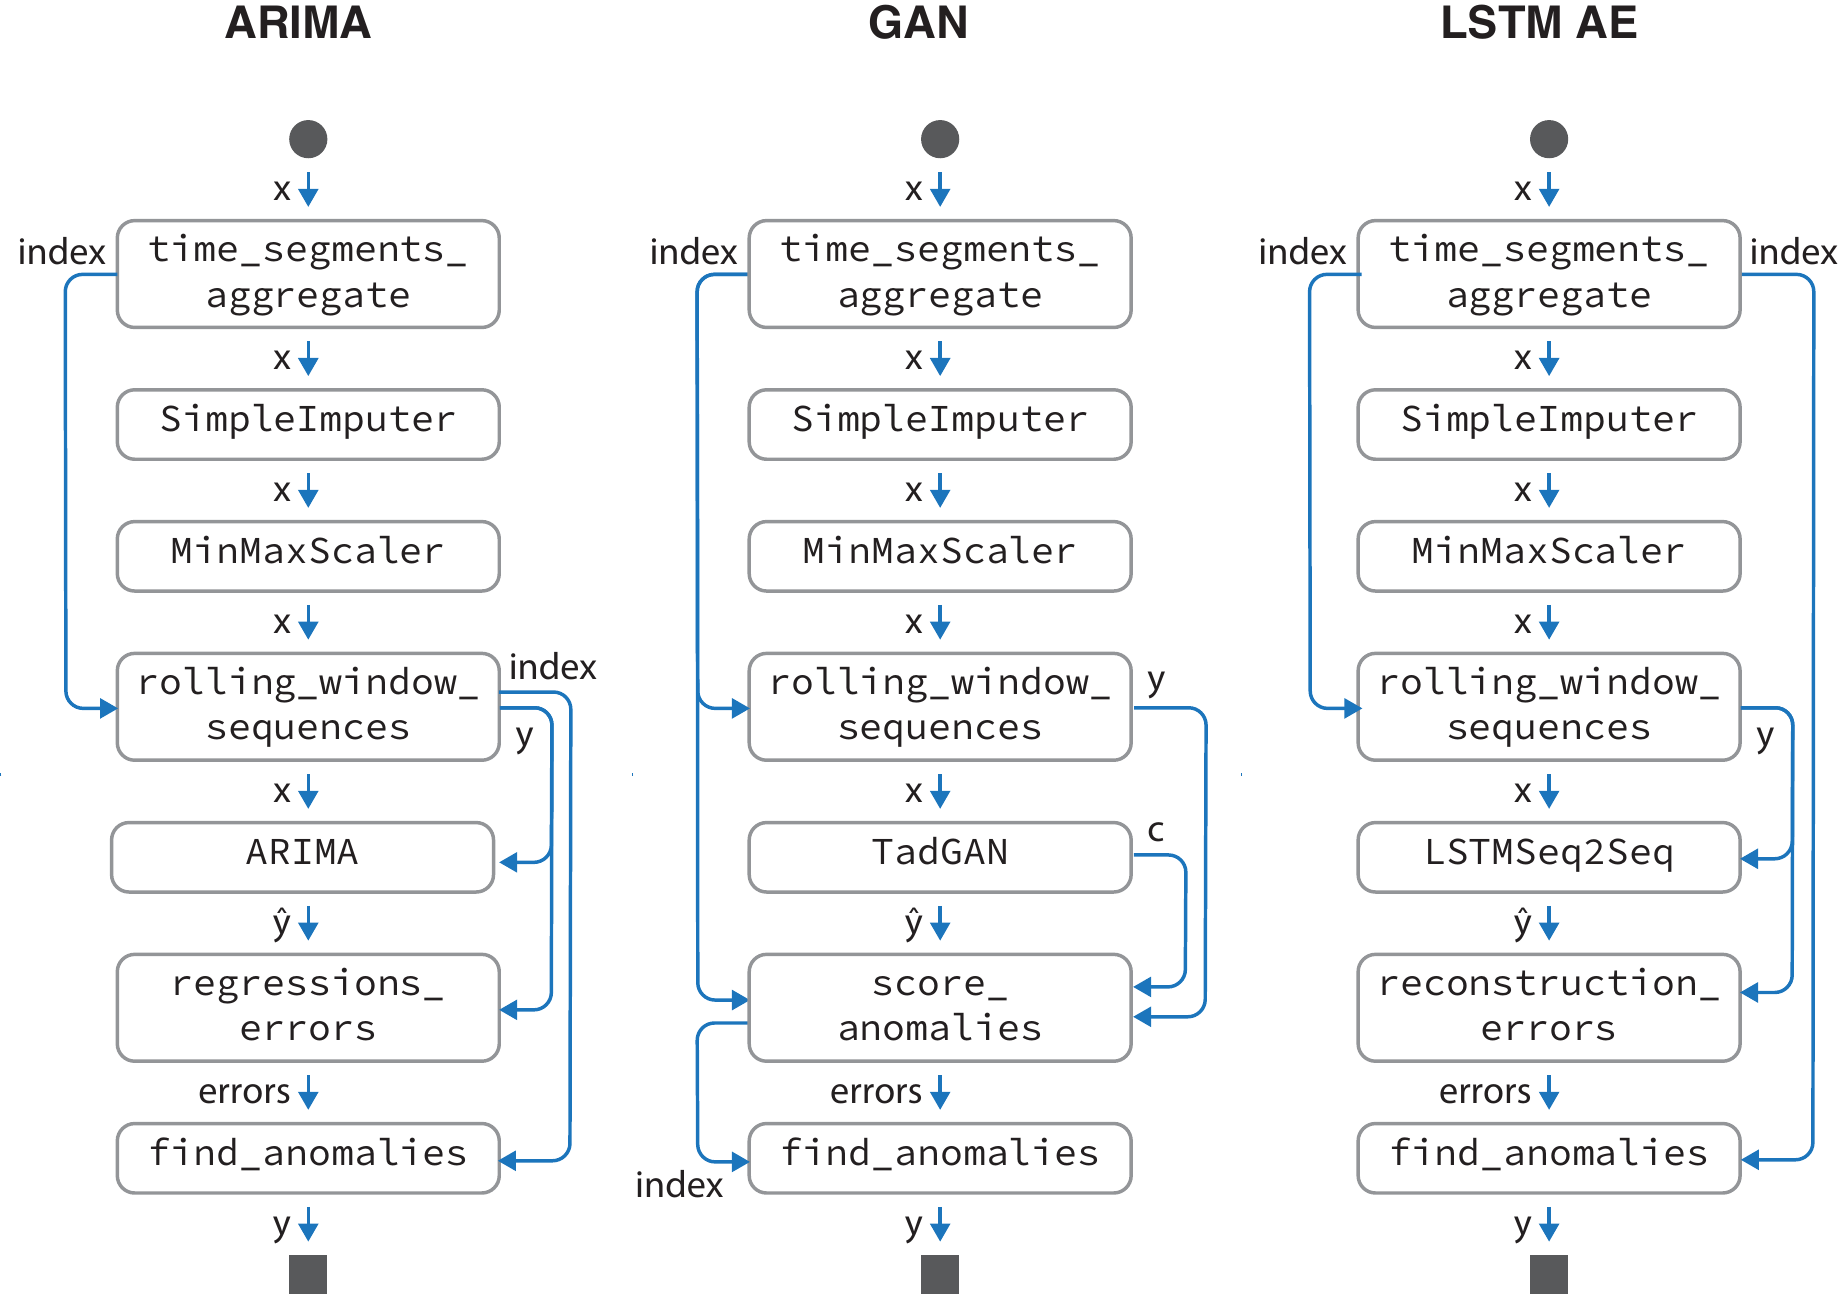}
\caption{Overview of the different anomaly detection pipelines} 
\label{fig:pipelines}
\end{figure}

As mentioned in section \ref{sec:pipelines} the current implementation of \textit{Orion} contains three distinct Machine Learning pipelines, all of which consist of multiple steps. The steps of each pipeline can be seen in figure \ref{fig:pipelines}.

\begin{figure}[ht]
    \centering
    \includegraphics[width=\linewidth]{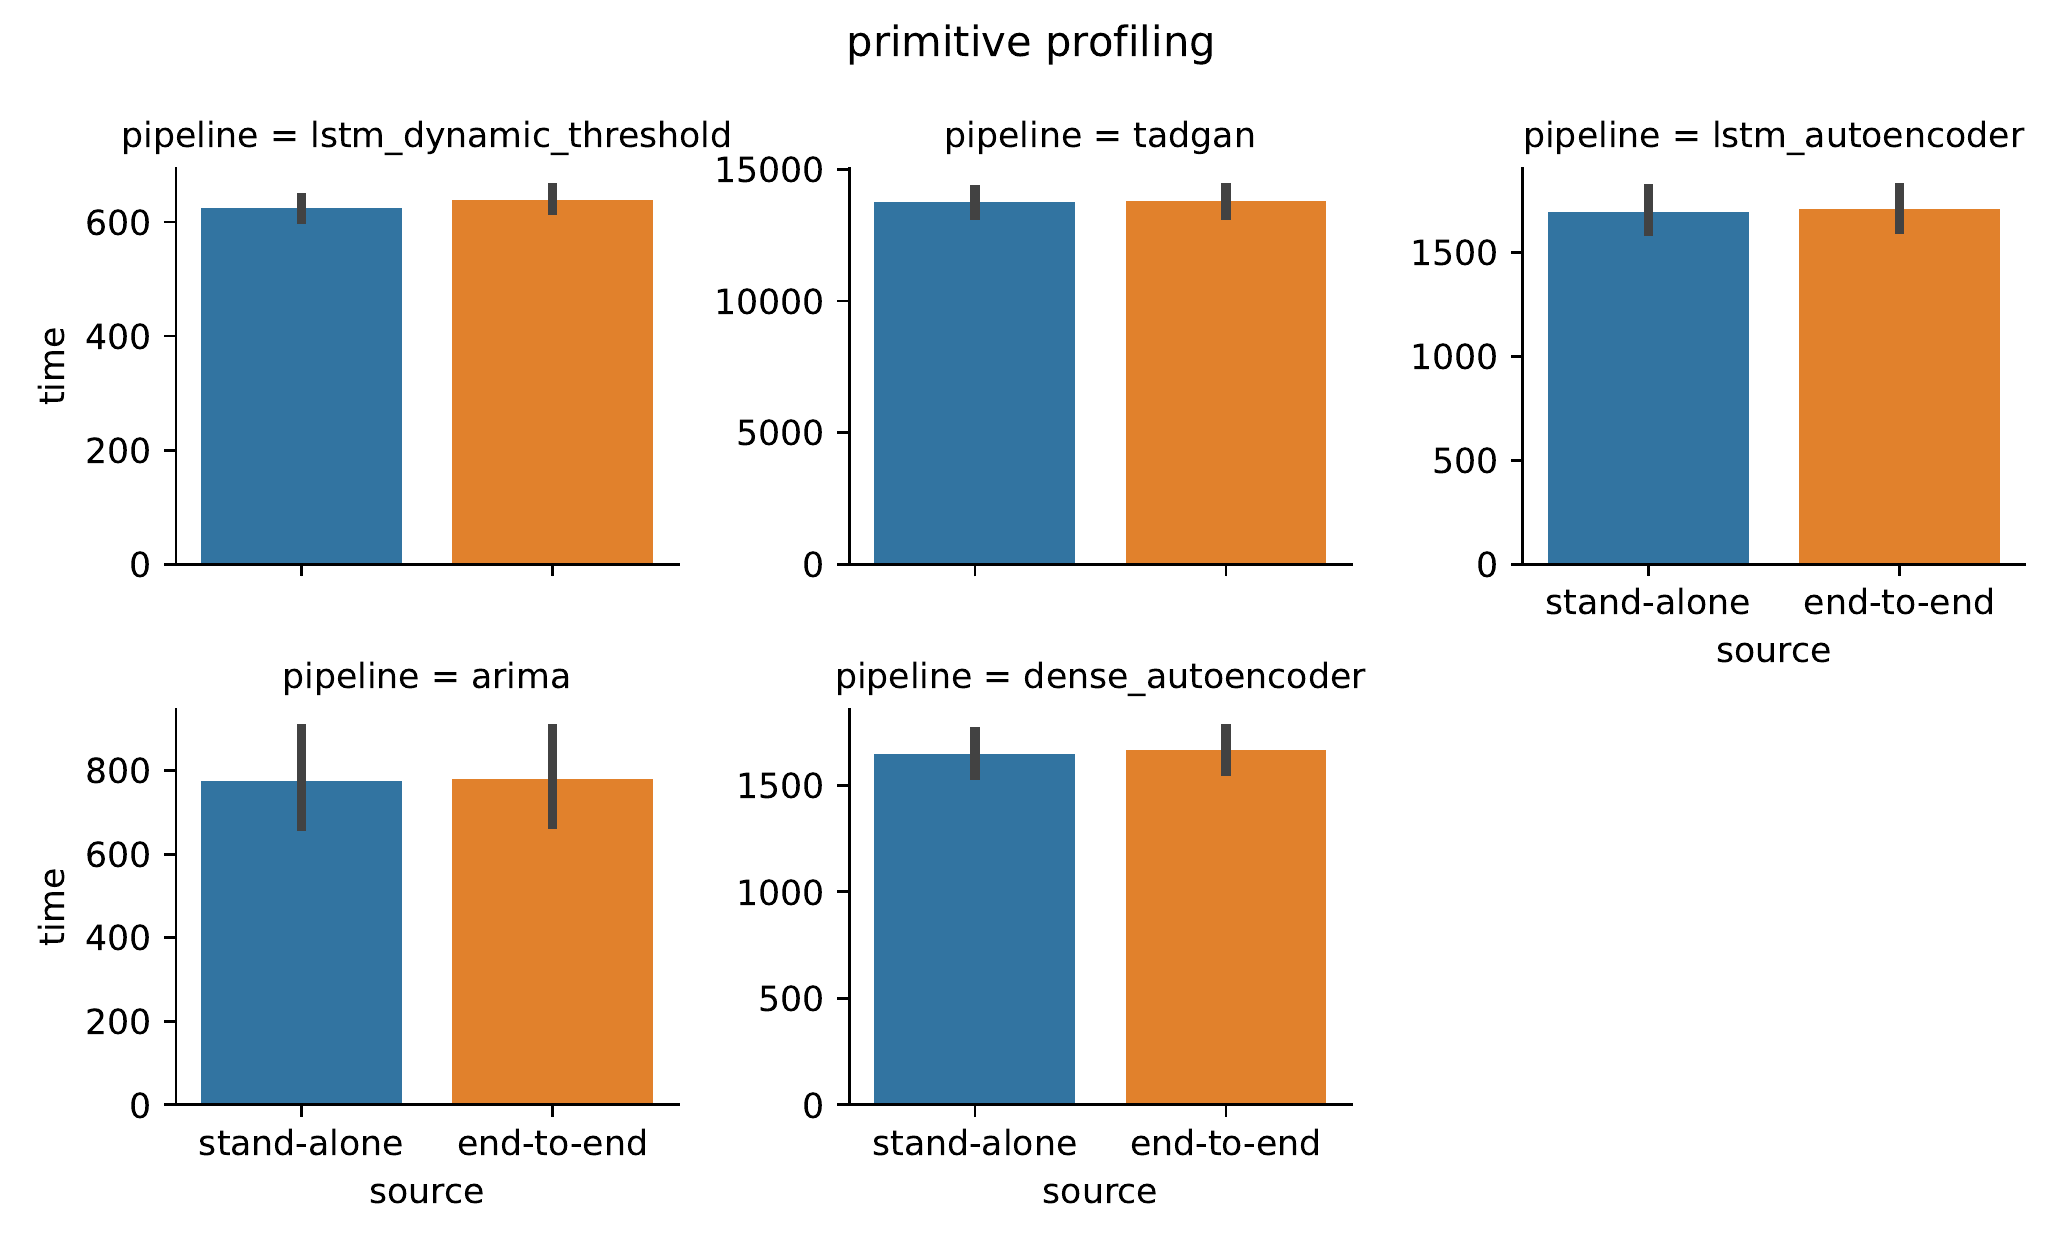}
    \caption{Running a pipeline end-to-end vs. standalone}
\end{figure}

\begin{figure*}[ht]
    \centering
    \includegraphics[width=0.9\linewidth]{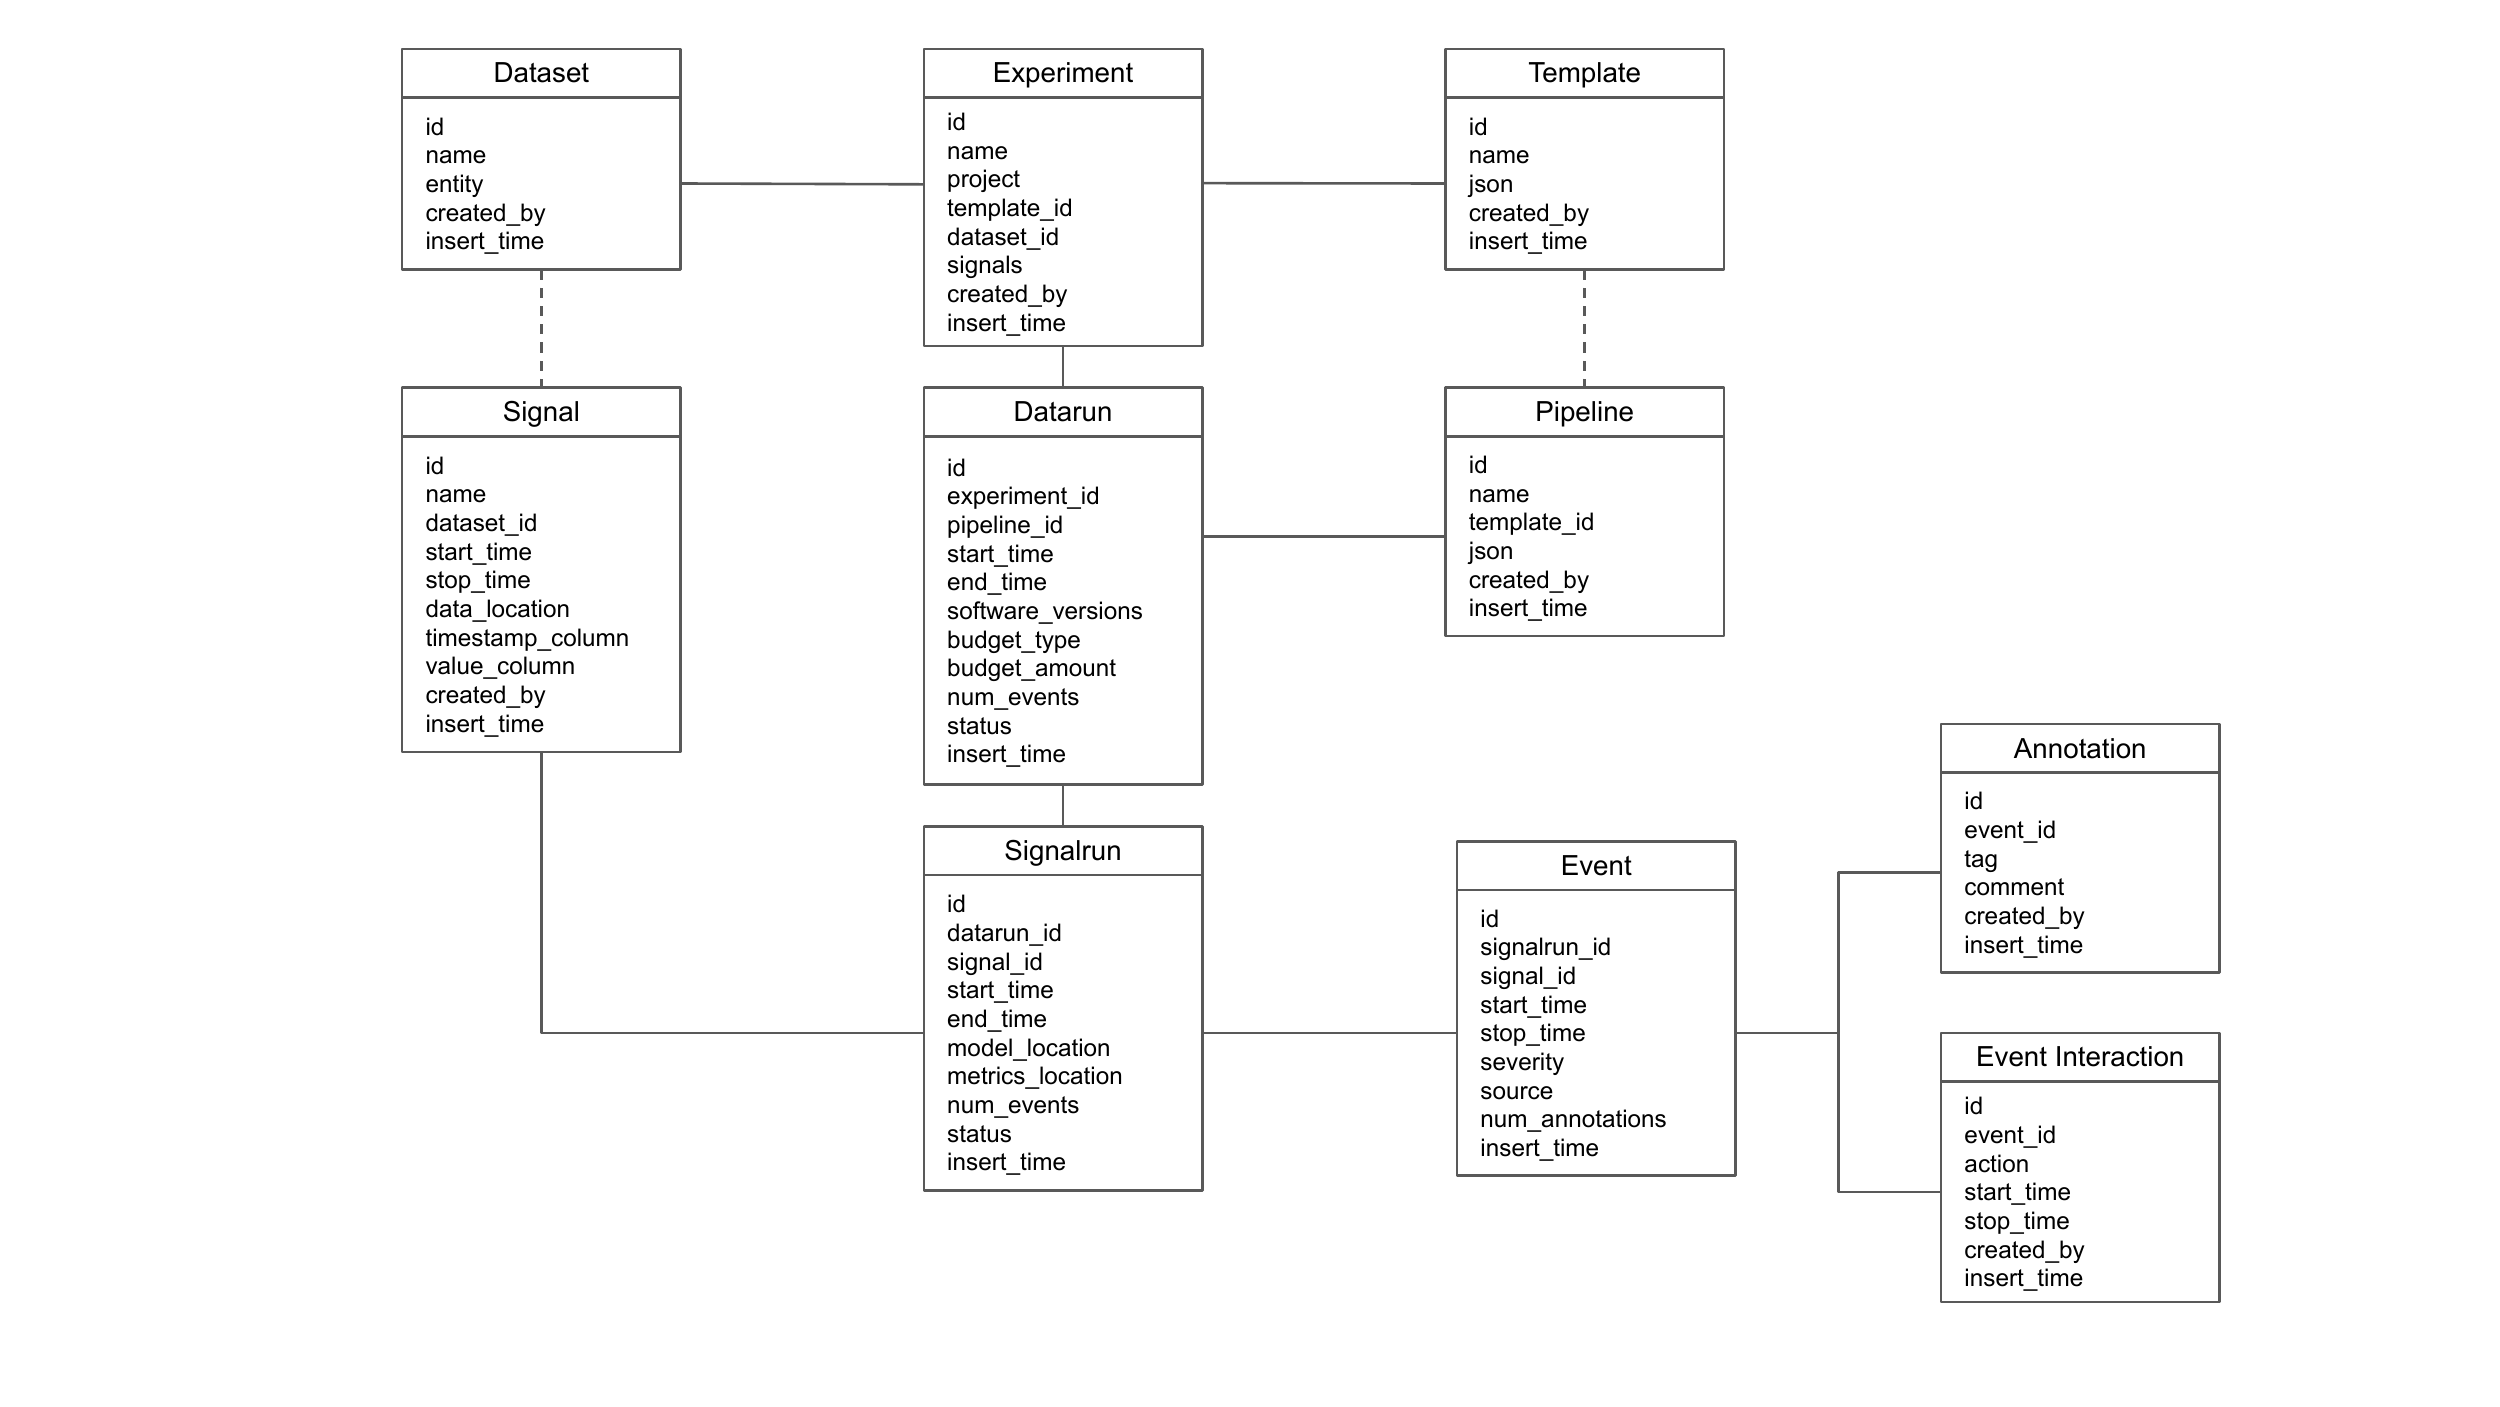}
    \caption{Database schema}
    \label{fig:db}
\end{figure*}

 \begin{table*}[!b]
 \caption{Precision, Recall and F1-Scores of pipelines}
 \begin{tabulary}{\textwidth}{*{2}{L}*{11}{c}}
 \toprule
  & & \multicolumn{2}{c}{NASA} & \multicolumn{4}{c}{Yahoo S5} & \multicolumn{5}{c}{NAB}  \\
   \cmidrule(r){3-4}\cmidrule(r){5-8}\cmidrule(r){9-13}
 \textbf{Variation} & & MSL & SMAP & A1 & A2 & A3 & A4 & Art & AWS & AdEx & Traf & Tweets\\
 \midrule
 \multirow{3}{*}{LSTM DT}
 & P    & 0.375 & 0.680 
        & 0.690 & 0.966 & 0.991 & 0.893 
        & 0.333 & 0.391 & 0.625 & 0.542 & 0.538 \\
 & R    & 0.667 & 0.761 
        & 0.815 & 0.985 & 0.589 & 0.510 
        & 0.500 & 0.600 & 0.909 & 0.929 & 0.636 \\
 & F1   & 0.480 & 0.718 
        & 0.747 & 0.975 & 0.739 & 0.649 
        & 0.400 & 0.474 & 0.741 & 0.684 &0.583 \\
 \hline
 \multirow{3}{*}{TadGAN}
 & P    & 0.451 & 0.573 
        & 0.592 & 0.792 & 0.764 & 0.575 
        & 0.625 & 0.625 & 0.625 & 0.391 & 0.559 \\
 & R    & 0.639 & 0.761 
        & 0.522 & 0.855 & 0.358 & 0.280 
        & 0.833 & 0.667 & 0.909 & 0.643 & 0.576 \\
 & F1   & 0.529 & 0.654 
        & 0.555 & 0.822 & 0.487 & 0.377 
        & 0.714 & 0.645 & 0.741 & 0.486 & 0.567 \\
 \hline
 \multirow{3}{*}{LSTM AE} 
 & P    & 0.450 & 0.635 
        & 0.629 & 0.833 & 0.931 & 0.711 
        & 0.667 & 0.840 & 0.533 & 0.412 & 0.640 \\
 & R    & 0.500 & 0.701 
        & 0.562 & 0.900 & 0.286 & 0.171 
        & 0.667 & 0.700 & 0.727 & 0.500 & 0.485 \\
 & F1   & 0.474 & 0.667 
        & 0.593 & 0.865 & 0.438 & 0.276 
        & 0.667 & 0.764 & 0.615 & 0.452 & 0.552 \\
 \hline
 \multirow{3}{*}{ARIMA} 
 & P    & 0.393 & 0.304 
        & 0.684 & 0.772 & 0.998 & 0.955 
        & 0.375 & 0.405 & 0.727 & 0.429 & 0.444 \\
 & R    & 0.306 & 0.313 
        & 0.815 & 0.865 & 0.643 & 0.533 
        & 0.500 & 0.567 & 0.727 & 0.429 & 0.606 \\
 & F1   & 0.344 & 0.309 
        & 0.744 & 0.816 & 0.782 & 0.684 
        & 0.429 & 0.472 & 0.727 & 0.429 & 0.513 \\
 \hline
 \multirow{3}{*}{Dense AE} 
 & P    & 0.567 & 0.712 
        & 0.719 & 0.955 & 0.975 & 0.586 
        & 0.600 & 0.846 & 0.667 & 0.529 & 0.600 \\
 & R    & 0.472 & 0.627 
        & 0.590 & 0.845 & 0.042 & 0.049 
        & 0.500 & 0.733 & 0.545 &  0.643 & 0.455 \\
 & F1   & 0.515 & 0.667 
        & 0.648 & 0.897 & 0.080 & 0.091 
        & 0.545 & 0.786 & 0.600 & 0.581 & 0.517 \\
 \hline
 \multirow{3}{*}{MS Azure} 
 & P    & \\
 & R    & \\
 & F1   & \\
 \bottomrule
 \end{tabulary}
 \label{tab:results_appendix}
 \end{table*}
